# Supplementary material for: Macroscopic phase separation of superconductivity and ferromagnetism in Sr0.5Ce0.5FBiS2-xSex revealed by muSR
Source: arXiv:1709.03632 source file (2017-09-12)
Supplement: Supplementary file 1 [file SUPPLEMENTARY_INFORMATION.pdf]

**SUPPLEMENTARY INFORMATION**

# Macroscopic phase separation of superconductivity and ferromagnetism in $Sr_{0.5}Ce_{0.5}FBiS_{2-x}Se_x$ revealed by μSR

A.M. Nikitin[1], V. Grinenko[2,3], R. Sarkar[2], J.-C. Orain[3], M. Salis[1], J. Henke[1], Y.K. Huang[1], H.-H. Klauss[2], A. Amato[3] and A. de Visser[1]

[1]*Van der Waals - Zeeman Institute, University of Amsterdam, 1098 XH Amsterdam, The Netherlands*
[2]*Institute of Solid State and Materials Physics, Technical University Dresden, 01062 Dresden, Germany*
[3]*Leibniz Institute for Solid State and Materials Research (IFW), 01069 Dresden, Germany*
[4]*Laboratory for Muon-Spin Spectroscopy, Paul Scherrer Institute, 5232 Villigen PSI, Switzerland*

## 1. Magnetic susceptibility and magnetization of $Sr_{0.5}Ce_{0.5}FBiSSe$

The magnetic susceptibility, $\chi(T)$, and the magnetization, $M(H)$, for $x = 1.0$ were measured in a Physical Properties Measurement System (PPMS) of Quantum Design down to 2.0 K on a bar-shaped sample ($1.0\times1.5\times5$ mm$^3$) with mass 50 mg. The inverse molar susceptibility $1/\chi_M$ measured in a field $B = 1$ T is a linear function of temperature in the range 70-300 K as shown in Fig. S1. The deduced effective moment, $p_{eff}$, has a value of 2.35 $\mu_B$/Ce and the paramagnetic Curie Weiss temperature $\theta_P$ is -28.1 K. These values are comparable to those reported in the literature: 2.29 $\mu_B$/Ce and $\theta_P$ = -8.2 K (Ref. 1). The value of $p_{eff}$ is smaller than the free-ion value 2.54 $\mu_B$ for trivalent Ce, which indicates the presence of crystalline electric field effects. The magnetization, measured at fixed temperatures in the range 2-50 K and fields up to 8 T, is shown in Fig. S2. At low temperatures the magnetization saturates in the high field region and attains the large value ~ 0.9 $\mu_B$/Ce at $T = 2$ K. The steep increase in low fields at $T = 2$ K corresponds to a spontaneous magnetization with a ferromagnetically ordered moment $m_0$ ~ 0.2 $\mu_B$/Ce.

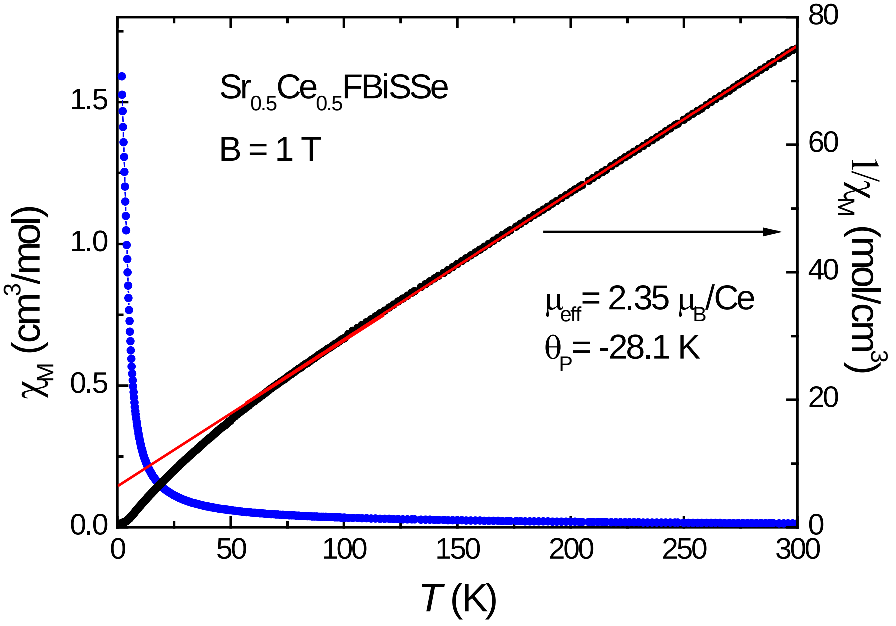


Fig. S1 Left axis: Molar dc-susceptibility of $Sr_{0.5}Ce_{0.5}FBiSSe$ measured in a field of 1 T (blue symbols). Right axis: $1/\chi_M$ (black symbols) and Curie-Weiss fit in the temperature range 70-300 K (red line).

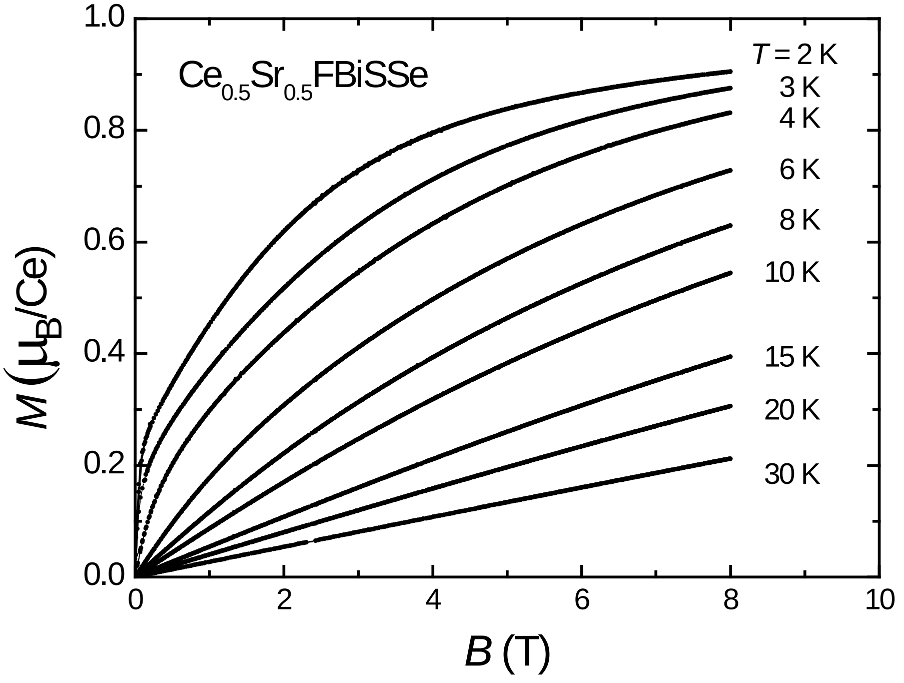


Fig. S2 Magnetization of $Sr_{0.5}Ce_{0.5}FBiSSe$ measured at the indicated temperatures.

**2. Specific heat of $Sr_{0.5}Ce_{0.5}FBiSSe$**

The specific heat for $x = 1.0$ was measured on a sample with a mass of 30 mg by the relaxation method using the Heat Capacity Option in the PPMS in the temperature range 2-300 K. In Fig. S3 we show the low temperature data ($T < 10$ K) in a plot of $c/T$ versus $T^2$. The large and broad peak is due to the ferromagnetic order. The Curie temperature is identified by the growing increase of $c/T$ at $T_C = 3.3$ K. The dashed linear line represents $c = \gamma T + \beta T^3$, where $\gamma$ and $\beta$ are the usual coefficients for the conduction electron and lattice contributions, respectively. The extracted values $\gamma = 22$ mJ/molK$^2$ and the Debye temperature $\theta_D = 180$ K are comparable to the values $\gamma = 12$ mJ/molK$^2$ and $\theta_D = 187$ K reported for $x = 0.5$ in Ref. 1. The magnetic entropy $S_m$ obtained after subtracting the electronic and lattice contributions is shown in the inset. $S_m$ saturates at 0.41×Rln2 at 10 K.

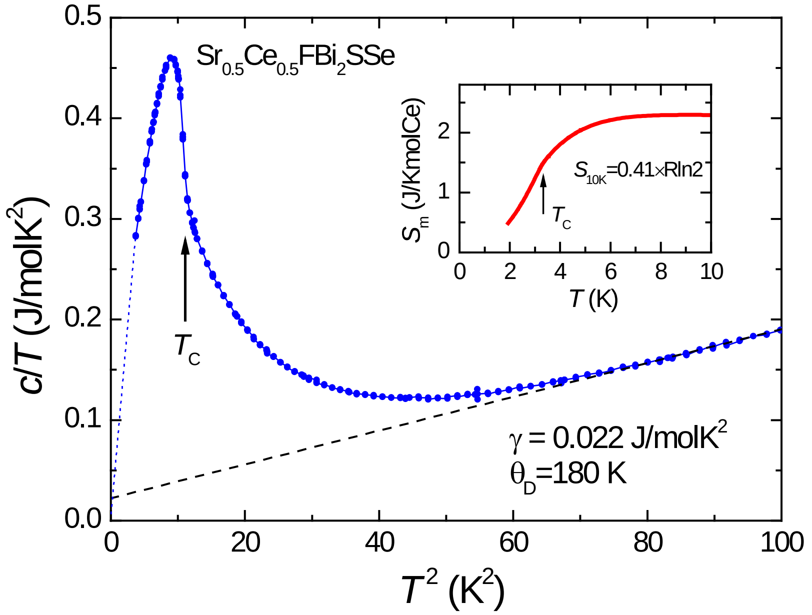


Figure S3. Specific heat of $Sr_{0.5}Ce_{0.5}FBiSSe$ in a plot of $c/T$ versus $T^2$. The dashed line represents $c = \gamma T + \beta T^3$. The inset shows the entropy associated with the magnetic transition. The arrows indicate the Curie temperature.

## 3. Ac susceptibility of $Sr_{0.5}Ce_{0.5}FBiSSe$

The ac-susceptibility, $\chi_{ac}$, was measured on a bar-shaped sample in a driving field of 1 Oe and a frequency $f$ = 1013 Hz in the PPMS in the temperature range 2-10 K. The zero-field cooled in-phase, $\chi'_{ac}$, and out-of-phase, $\chi''_{ac}$, signal are shown in Fig. S4. The increase of $\chi'_{ac}$ below ~ 4 K is due to magnetic order. The Curie point as determined by the specific heat data (Fig. S3) is indicated by the arrow. The diamagnetic signal is due to superconductivity, with a transition temperature $T_{sc}$ = 2.92 K as determined by the midpoint of the transition. Close to this temperature $\chi''_{ac}$ peaks. The size of the diamagnetic signal measured in 1 Oe corresponds to a superconducting volume fraction of ~ 70 %. Data taken in small applied fields up to 0.075 T show the depression of superconductivity.

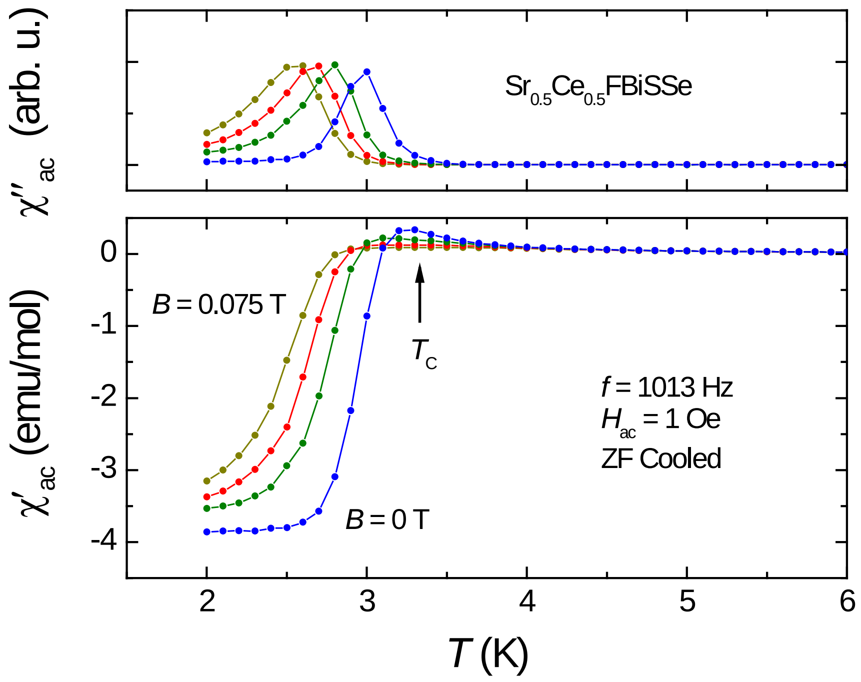


Fig. S4 Ac susceptibility of $Sr_{0.5}Ce_{0.5}FBiSSe$ measured in zero field and small applied fields from right to left $B$ = 0, 0.025, 0.050 and 0.075 T.

## 4. Electrical resistivity and upper critical field of $Sr_{0.5}Ce_{0.5}FBiSSe$

The electrical resistivity, ρ, was measured in the PPMS in the temperature range 2-300 K. Data were taken on a bar-shaped sample with an excitation current of 1 mA. The results are shown in Fig. S5. The resistivity has a metallic temperature variation. Superconductivity (see lower inset) has an onset temperature of 3.70 K, while zero resistance is observed at 2.89 K, which is close to $T_{sc}$ determined by ac-susceptibility. In the lower inset the superconducting transition in fields between 0 and 1.5 T is reported. The upper critical field, $B_{c2}$, extracted from resistivity data in fixed fields is shown in the upper inset. Here we follow the same procedure as in Ref. 1 and take data points at 90% of the normal state resistivity value at 4 K ($0.9\times\rho_N$) indicated by the horizontal dashed line in the lower inset. We remark the superconducting transition broadens considerably in field and the $0.9\times\rho_N$ criterion results in an overestimation of $B_{c2}$. The red line shows a comparison of $B_{c2}(T)$ with the Werthamer, Helfand and Hohenberg (WHH) expression for a weak-coupling spin-singlet orbital-limited superconductor (Ref. 2).

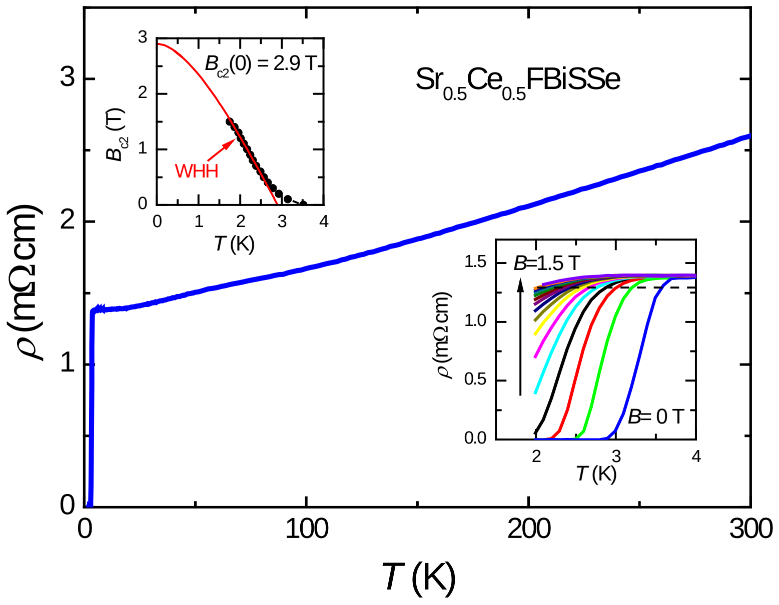


Fig. S5 Electrical resistivity of $Sr_{0.5}Ce_{0.5}FBiSSe$ as a function of temperature. Lower inset: ρ(*T*) in fixed magnetic fields between 0 and 1.5 T with steps of 0.1 T. The horizontal dashed line represents $0.9\times\rho_N$. Upper inset: Upper critical field $B_{c2}(T)$ (solid symbols). The red line is a comparison with the WHH model.

## 5. Low field magnetization and lower critical field of $Sr_{0.5}Ce_{0.5}FBiSSe$

In order to investigate the superconducting state the low field magnetization $M(H)$ was measured in the PPMS in the temperature range 1.9 - 4 K, see Fig. S6(a). Upon cooling below 4 K the slope $dM/dH$ first increases due to ferromagnetic order. Below 2.8 K a diamagnetic signal is observed. In the superconducting state, at low fields $M = - H$ and the field where $M(H)$ deviates from a linear function is taken as the lower critical field $H_{c1}$. $H_{c1}(T)$ follows the usual temperature variation $H_{c1}(T) = H_{c1}(0)\ (1-(T/T_{sc})^2)$ with $H_{c1}(0) = 6$ Oe as shown in Fig. S6(c). In Fig. S6(b) we show a typical magnetic hysteresis loop measured at $T = 2.0$ K. The superconducting loop is superposed on a ferromagnetic loop.

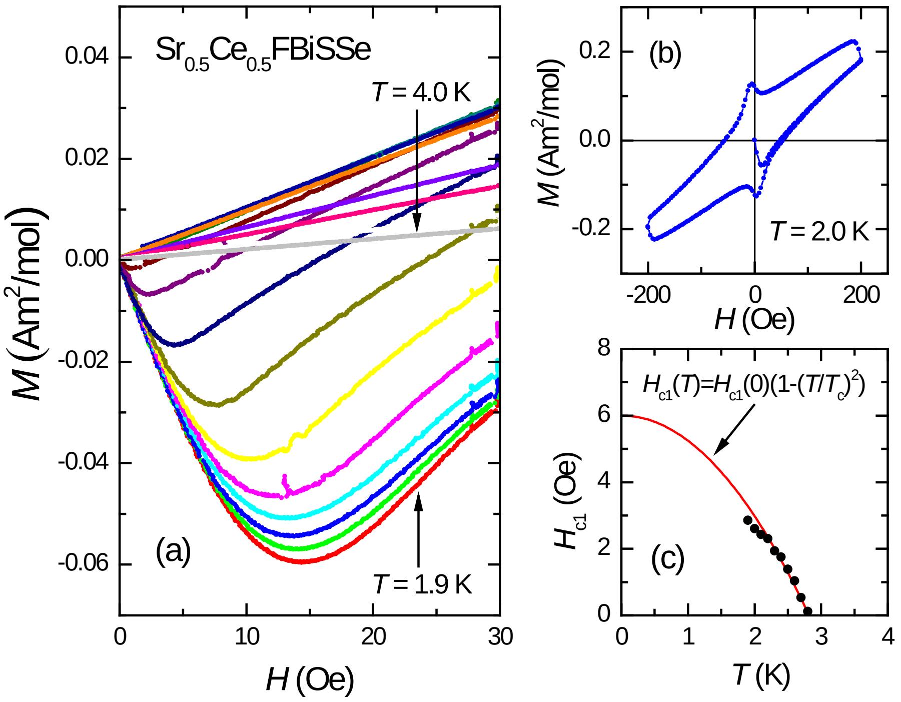


Fig. S6 (a) Low field magnetization of $Sr_{0.5}Ce_{0.5}FBiSSe$ at temperatures of 1.9 - 3.2 K in steps of 0.1 K, and at 3.4, 3.5, 3.75 and 4.0 K. (b) Superposed ferromagnetic and superconducting magnetization loop at 2.0 K. (c) Lower critical field $H_{c1}(T)$ (solid symbols). The red line represent the standard quadratic temperature variation of $H_{c1}$.

## References

[1] G.S. Thakur, G. Fuchs, K. Nenkov, Z. Haque, L.C. Gupta and A.K. Ganguli, Sci. Reports **6**, 37527 (2016).
[2] N.R. Werthamer, E. Helfand and P.C. Hohenberg, Phys. Rev. **147**, 295 (1966).
